# Supplementary material for: The Effect of Geometry, Spin and Orbital Optimization in Achieving Accurate, Fully-Correlated Results for Iron-Sulfur Cubanes
Source: arXiv:2105.01754 ancillary file (2021-05-07)
Supplement: Supplementary file 1 [file supp.pdf]

# Supporting Information for “The Effect of Geometry, Spin and Orbital Optimization in Achieving Accurate, Fully-Correlated Results for Iron-Sulfur Cubanes”

Carlos Mejuto-Zaera,<sup>1,2,\*</sup> Demeter Tzeli,<sup>3</sup> David Williams-Young,<sup>2</sup> Norm M. Tubman,<sup>4,†</sup> Mikuláš Matoušek,<sup>5</sup> Jiri Brabec,<sup>5</sup> Libor Veis,<sup>5,‡</sup> Sotiris S. Xantheas,<sup>6,7,§</sup> and Wibe A. de Jong<sup>2,¶</sup>

<sup>1</sup>*University of California, Berkeley, California 94720, United States*

<sup>2</sup>*Computational Research Division, Lawrence Berkeley National Laboratory, Berkeley, CA 94720, USA*

<sup>3</sup>*Quantum Theoretical and Physical Chemistry Institute,  
National Hellenic Research Foundation, Athens 11635, Greece*

<sup>4</sup>*Quantum Artificial Intelligence Lab. (QuAIL), Exploration Technology Directorate,  
NASA Ames Research Center, Moffett Field, CA 94035, USA*

<sup>5</sup>*J. Heyrovský Institute of Physical Chemistry, Academy of Sciences of the Czech Republic,  
v.v.i., Dolejškova 3, 18223 Prague 8, Czech Republic*

<sup>6</sup>*Advanced Computing, Mathematics and Data Division,  
Pacific Northwest National Laboratory, 902 Battelle Boulevard,  
P.O. Box 999, MS K1-83, Richland, WA 99352, USA*

<sup>7</sup>*Department of Chemistry, University of Washington, Seattle, WA 98185, USA*

(Dated: May 7, 2021)

In this Supporting Information (SI), we include

1. a description of the adaptive sampling configuration interaction (ASCI) algorithm used as solvers for the CASSCF optimization, as well as the introduction of the Spin Pure ASCI (SP-ASCI) approach to ensure spin-conservation after within the ASCI Hilbert space truncation,
2. five geometries of the  $[\text{Fe}_3\text{S}_4(\text{SCH}_3)_3]^{-2}$  cluster (i.e. one Fe atom less than the clusters in the main paper), which served as initial tests for the ROHF and CASSCF calculations,
3. details on the ROHF starting point calculations, including the orbital localization,
4. ROHF and CASSCF energies for different spin states of the five  $\text{Fe}_3$  geometries,
5. a brief analysis of the orbital component of the CASSCF molecular orbitals in the  $\text{Fe}_4$  clusters,
6. ROHF and CASSCF energies for the 2R  $\text{Fe}_4$  cluster, using the def2-SVP basis set, equivalent to the basis set used in Ref. [1],
7. a brief discussion on performing the orbital optimization with different basis sets.

## I. ASCI SOLVERS FOR CASSCF

### A. ASCI and ASCI-SCF

The ASCI approach is an exceptionally efficient selected configuration interaction (SCI) algorithm for ground states. Essentially, given a many-body Hamiltonian  $H$  in second quantization, it finds an optimal Hilbert space truncation  $\mathcal{T}$  of specified size  $|\mathcal{T}|$ , to approximate the ground state wave function  $|\Psi_0\rangle$  of  $H$ . This truncation  $\mathcal{T}$  is a set of Slater determinants  $|D_\alpha\rangle$ , and is optimal in the sense that it includes almost all important determinants of  $|\Psi_0\rangle$ , i.e. those with the largest absolute coefficients. These determinants are found iteratively, following a series of Compute-Explore-Rank-Truncate steps: Given a proposed truncation  $\mathcal{T}^i$  in the  $i$ -th iteration, the ground state of  $H$  projected onto  $\mathcal{T}^i$  is Computed. This means that we determine the expansion coefficients in  $|\Psi_0^i\rangle = \sum_{\beta \in \mathcal{T}^i} a_\beta^i |D_\beta\rangle$ , and the corresponding energy  $E_0^i$ . Then, sections of the Hilbert space beyond  $\mathcal{T}^i$  are Explored, by finding the single and double excitation determinants from the most important determinants in  $\mathcal{T}^i$ . These newly found determinants  $|D_\alpha\rangle \in \mathcal{T}_{SD}^i$  are Ranked

---

\* carlos\_mejutozaera@berkeley.edu

† norman.m.tubman@nasa.gov

‡ libor.veis@jh-inst.cas.cz

§ sotiris.xantheas@pnnl.gov

¶ WAdJong@lbl.gov

with the determinants in  $\mathcal{T}^i$ , by estimating their coefficients  $a_\alpha^i$  in the ground state wave function perturbatively [2–4], according to

$$a_\alpha^i \approx \frac{\sum_{\beta \in \mathcal{T}^i} H_{\alpha,\beta} a_\beta}{E_0^i - H_{\alpha,\alpha}}, \text{ for } \alpha \in \mathcal{T}_{SD}^i \quad (1)$$

where we have introduced the Hamiltonian matrix elements  $H_{\alpha,\beta} = \langle D_\alpha | H | D_\beta \rangle$ . We finally Truncate the set  $\mathcal{T}^i \cup \mathcal{T}_{SD}^i$ , keeping only the  $|\mathcal{T}|$  determinants with largest computed or estimated coefficients  $a_\alpha^i$ , defining the new truncation  $\mathcal{T}^{i+1}$ . The method is repeated until the ground state energy  $E_0^i$  converges within a chosen threshold.

The identity of the determinants in the truncation  $\mathcal{T}$  depends on the single-particle orbital basis used. The ASCI calculations typically start in some mean-field orbital basis, such as Hartree-Fock (HF) orbitals. Still, the orbitals can be improved to provide more compact wave function representations during the ASCI iterations. The most simple approach corresponds to computing a natural orbital basis [5–8] for the current ASCI ground state approximation. A more sophisticated approach relies on performing a CASSCF orbital optimization using ASCI as approximate solver. This has been recently applied to CASSCF calculations with large active spaces in transition metal systems [9, 10], allowing the use of larger active spaces than what is commonly possible.

ASCI and ASCI-SCF have been shown to provide near full CI (FCI) accuracy for ground state energies and spectral functions for a wide variety of challenging, strongly correlated molecular and extended systems [9, 11–18]. As a rule of thumb, we expect ASCI to work well in systems which (i) have a dense two-body interaction tensor  $U_{p,q,r,s}$ , giving each determinant a large number of double excitations and thus making the exploration step more thorough, (ii) have a ground state which can be effectively described by a computationally manageable number of determinants, i.e. a few million. The latter condition is hard to judge *a priori* for a given Hamiltonian, but is typically met for ground states with a moderate number of active orbitals, i.e. less than 50. This number can be estimated for a given problem by computing the eigenvalues of the one-particle reduced density matrix (1-RDM) using a preliminary, more approximate, ground state description.

Here, we used the ASCI-SCF approach to optimize the single-particle orbital basis, and thus investigate its effect on the ordering of the low energy, low spin states of the iron-sulfur clusters. We use the BFGS optimization described in detail in Ref. [9], computing 1- and 2-RDMs from the ASCI wave function and considering orbital rotations between inactive-active, inactive-secondary, active-secondary and active-active orbitals. This final class of rotations is important when using ASCI as CAS solver approximation, since the lack of a complete full CI description allows for energy lowering with rotations within the active space.

## B. Spin Pure ASCI Mimicking CSFs

While the ASCI truncation has been shown to give highly accurate ground state approximations, by its very nature it is susceptible to breaking system symmetries. Given an operator  $O$  commuting with the full system Hamiltonian, the method described above does not guarantee that the projected  $O$  and  $H$  into the ASCI truncation  $\mathcal{T}$  will also commute. For non-relativistic quantum chemical systems, arguably the most prominent example is the conservation of the total electron spin  $O = S_{tot}^2$ , with its violation leading to spin contamination. While for the systems considered in previous studies [9, 11–18], spin contamination has not been significant, in molecules of strong magnetic character, such as the iron-sulfur clusters considered here, this is more likely to be an issue. Indeed, we have observed drastic amounts of spin contamination when using plain ASCI even in modest active spaces, such as those containing only Fe-3d orbitals. In order to produce reliable energies and orbitals for states of well-defined electronic spin, modifying the original ASCI approach was necessary.

We introduce here a modification of the ASCI Search and ground state Computation steps to ensure that the approximate ground states have a well-defined, and targeted total electronic spin. These modifications are related to previously reported approaches to deal with spin contamination in selected CI based computations [19–21], but are adapted to best suit the ASCI framework.

The main obstacle to ensure that the Search step produces truncations preserving spin symmetry relies on the fact that Slater determinants are generally not eigenstates of the total spin operator  $S^2$  [22]. Thus, the main idea is to formulate the ASCI search not in terms of single determinants, but of determinant families, such that these families can produce states of definite total spin through linear combinations. To this end, we collect determinants in terms of configuration state function (CSF) families. Given a Slater determinant, the CSF family to which it belongs is determined by its orbital occupation. All determinants with the same orbitals being doubly and singly occupied belong to the same CSF family. Thus, given a fix active space ( $N_{el}$  e,  $N_{orb}$  o) and spin projection  $M = \langle S_{z,tot} \rangle$ , the determinants within a CSF family differ only in the distribution of spins up and down in their singly occupied orbitals, comprising all possible such distributions. For instance, the CSF family of  $|2, \uparrow, \downarrow, 0, \uparrow, 2\rangle$ , corresponds to

$\{|2, \downarrow, \uparrow, 0, \uparrow, 2\rangle, |2, \uparrow, \downarrow, 0, \uparrow, 2\rangle, |2, \uparrow, \uparrow, 0, \downarrow, 2\rangle\}$ , and all possible states with occupation  $|2, 1, 1, 0, 1, 2\rangle$  and defined total spin can be built from linear combinations of those three determinants [22].

Thus, at the end of the ASCI Search step we group the determinants found, both in  $\mathcal{T}^i$  and  $\mathcal{T}_{SD}^i$ , in their respective CSF families. Instead of ranking determinants, we rank CSF families, their collective coefficients defined as the sum of the absolute values of the coefficients of its constituent determinants. Determinants which would formally be part of the CSF family, but which were not found by ASCI yet, contribute zero to the collective coefficient. After the ranking, the new truncation  $\mathcal{T}^{i+1}$  is built by including full CSF families, including those determinants not found previously, following the ranking, until the maximal size  $|\mathcal{T}|$  is reached.

Formulating the ASCI Search in terms of CSF families ensures that the eigenstates of the truncated Hamiltonian will have a definite spin. Still, there is no guarantee that the ground state of the truncated Hamiltonians, which drive the ASCI search through Eq. (1), will be of the particular spin state of interest. In this work, we want to study the lowest possible spin state for different spin projections  $M$ , and in order to do so we introduce a final modification, this time in the Compute step. Instead of diagonalizing the truncated Hamiltonian  $H$ , we diagonalize  $H' = H + \lambda S^2$ , where  $\lambda$  is a positive penalty factor. By choosing  $\lambda$  such that it is comparable to the energy gap between the Hamiltonian eigenstates, we select the eigenstates of smallest total spin as effective ground states. We then use their actual energy, i.e.  $\langle \Psi_0^i | H | \Psi_0^i \rangle^1$ , for  $E_0^i$  in Eq. (1). This spin penalty and the CSF based search avoid spin contamination and allow targeting low spin states within the ASCI truncation. We refer to this new spin on ASCI as SP-ASCI, or spin pure ASCI.

For context, we want to relate SP-ASCI to previous work. We note that the formulation of the Search in terms of CSF families is similar to the work in Ref. [20]. There, after a converged selected CI approach provides with a Hilbert space truncation, the authors propose extending the truncation by completing all CSF families present at the end of the selected CI. For the iron-sulfur clusters considered here, this would result in a prohibitive increase of the truncation in the final step, forcing the use of insufficiently large truncations during the ASCI iterations. In our approach, by formulating instead the iterative Hilbert space exploration in terms of the CSF families directly, we keep only the most important CSF families at any given point, and keep thus in the spirit of ASCI the number of determinants in the final truncation manageable, i.e. a few million. The advantages and disadvantages of different spin penalties in the Hamiltonian for determinant-based CI have been studied previously, c.f. Ref. [19]. Here we choose the linear penalty function for its computational simplicity, and because we are only interested in the smallest total spin state for each spin projection  $M$ . Finally, the most compact way to perform a pure CSF based ASCI would be to use CSFs themselves, instead of determinants, as the basic units of the ASCI wave function expansion, c.f. Ref. [21]. Here, we chose to explore this hybrid determinant/CSF formulation for simplicity, both in terms of modifying the previously existing ASCI code, and because both the Search and Hamiltonian construction steps are easier to formulate in terms of determinants.

### C. On converging ASCI-SCF and SP-ASCI-SCF

As pointed out in the main text, when performing CASSCF optimizations in challenging systems such as the iron-sulfur clusters, it is crucial to keep in mind that one is not guaranteed to find the actual global minimum of the optimization process. Instead, most likely the CASSCF process will converge to a stable local minimum, and there is typically no way to identify this as such, other than escaping the minimum in some way.

Within ASCI-SCF, one can try to escape local minima by “shaking” previously converged orbitals. In the original ASCI-SCF study [9], it was suggested to perform an inexpensive (small determinant truncation) ASCI-SCF calculation starting from the converged orbitals, on a different spin state (e.g. on a triplet, if the optimization of interest is being done on a singlet). A subsequent ASCI-SCF in the spin state of interest can overcome a previous local minimum. While we have employed this strategy in this work, the SP-ASCI approach allows for an orthogonal “shake”, without needing to change the spin state of the system: one can perform an inexpensive ASCI-SCF calculation on the same spin state, but without grouping the determinants by CSF families. For the iron-sulfur clusters of interest in this work, this results in wave functions with significant spin contamination, and hence different character, such that the single particle orbitals get also kicked out of their local minimum. We have performed cycles of consecutive orbital optimization and brief “shakings”, until the (SP)-ASCI-SCF energy converges to within  $\sim 1$  mHa. Still, while this strategy allows to avoid some local minima, it does not guarantee reaching the global minimum of the CASSCF optimization.

---

<sup>1</sup> Here, it is worth noting that the truncated  $H$  and  $S^2$  do commute, thanks to formulating the truncation in terms of CSF families.

## II. $\text{Fe}_3$ GEOMETRIES

Further, we present results, both at the ROHF and FCI/DMRG-CASSCF level for five different  $[\text{Fe}_3\text{S}_4(\text{SCH}_3)_3]^{-2}$  clusters, which served as initial test cases for our calculations. The corresponding average oxidation number of the Fe atoms in this clusters is +3, and the highest spin multiplicity in the Fe-d manifold is  $2S + 1 = 16$  (c.f. with  $2S + 1 = 19$  in the  $\text{Fe}_4$  clusters in the main paper, and average oxidation number of +2.5). The five geometries we consider, which we label 1A-E, were optimized for different spin states using broken-symmetry DFT (BS-DFT) with the TPPSh functional and the mixed aug-cc-pVDZ (Fe, S) and cc-pVDZ (H,C) basis set. We report a summary of cluster labels and targeted spin states in Tab. S1, including the  $\text{Fe}_4$  clusters for completeness. This table also includes the BS-DFT energies, as well as the ROHF energies for the high-spin state (HS). We further include an accompanying .zip file with the geometries of all 8 clusters.

| Cluster                 | $2S + 1$ | BS-DFT       | HS-ROHF ( $2S + 1$ ) |
|-------------------------|----------|--------------|----------------------|
| 1A ( $\text{Fe}_3$ )    | 6        | -6699.031569 | -6689.334426 (16)    |
| 1B ( $\text{Fe}_3$ )    | 4        | -6699.022110 | -6689.283679 (16)    |
| 1C ( $\text{Fe}_3$ )    | 2        | -6699.002427 | -6689.271816 (16)    |
| 1D ( $\text{Fe}_3$ )    | 2        | -6698.998914 | -6689.290452 (16)    |
| 1E ( $\text{Fe}_3$ )    | 16       | -6699.005959 | -6689.363419 (16)    |
| 2A ( $\text{Fe}_4$ )    | 19       | -8401.048191 | -8389.083540 (19)    |
| 2B ( $\text{Fe}_4$ )    | 1        | -8401.092653 | -8389.026178 (19)    |
| 2C ( $\text{Fe}_4$ )    | 1        | -8401.092522 | -8389.024431 (19)    |
| 2R[1] ( $\text{Fe}_4$ ) | —        | —            | -8388.979087 (19)    |

TABLE S1: Summary table relating the  $[\text{Fe}_x\text{S}_4(\text{SMe})_x]^{-2}$  cluster labels to their geometries. Each geometry was found by performing a BS-DFT optimization with different target spin states. We considered 5 geometries for the  $x = 3$  clusters (1A-E), three geometries for the  $x = 4$  clusters. The BS-DFT calculations used a mixed aug-cc-pVDZ (Fe, S) cc-pVDZ (C, H) basis set and the TPSSh functional. We further include the  $x = 4$  geometry in Ref. [1] in our study as reference point. We further show the ROHF energies for the high spin (HS) states in each cluster geometry, which we localized to use as starting point for the CASSCF orbital optimizations.

## III. ROHF STARTING POINTS

As starting points for the orbital optimizations of the  $[\text{Fe}_x\text{S}_4(\text{SCH}_3)_x]^{-2}$  clusters ( $x = 3, 4$ ), we performed restricted open-shell Hartree-Fock (ROHF) calculations on high-spin (HS) states of the different systems. This corresponds to  $2S + 1 = 16$  and  $2S + 1 = 19$  for the  $\text{Fe}_3$  and  $\text{Fe}_4$  clusters respectively. The reason behind this choice, even when experimental and computational evidence (including this work) suggest that the most stable configurations are low spin, relies on the character of the ROHF orbitals. While it is true that the ground state of these clusters are low-spin in nature, they present a high number of singly occupied orbitals, namely the Fe-3d ones. The low spin configuration is achieved through magnetic coupling of these single electrons, another manifestation of the intrinsically many-body, i.e. strongly correlated, nature of their electronic structure. A low spin ROHF solution would naturally leave most if not all electrons paired, since it is a single determinant solution, and would thus provide a poor starting point for the correlated CASSCF calculations.

As an evidence of this fact, in Tab. S2 we report the ROHF energies for the HS states (the ones used as starting points for the CASSCF calculations), as well as ROHF energies for the spin states for which the different cluster geometries were optimized. We further report unrestricted Hartree Fock (UHF)<sup>2</sup> energies for comparison. The same information for the  $\text{Fe}_3$  clusters is represented graphically in Fig. S1. We observe significant energy differences for the various geometries, which carry on to the many-body level of theory.

The HS ROHF energies are significantly lower than the lower spin ones, indicating them as a better variational starting point, besides the physical arguments previously discussed. The question arises whether it would be possible to improve upon the low spin ROHF energies, by sequentially lowering the spin from the HS ROHF orbitals. We tested this by using the HS ROHF orbitals in the 1E geometry as starting point for a  $2S + 1 = 14$  ROHF calculation,

<sup>2</sup> Although the UHF energies are generally lower than the ROHF ones except for the high spin states, as they should, we do not use

them for the CASSCF since our CASSCF code assumes restricted orbitals.

| cluster | Target Spin | High Spin | ROHF (Target Spin) | UHF (Target Spin) | UHF (High Spin) | ROHF (High Spin) |
|---------|-------------|-----------|--------------------|-------------------|-----------------|------------------|
| 1A      | 6           | 16        | -6688.824963       | -6689.121985      | -6689.364489    | -6689.334426     |
| 1B      | 4           | 16        | -6688.713617       | -6689.289696      | -6689.316601    | -6689.283679     |
| 1C      | 2           | 16        | -6688.673904       | -6689.169108      | -6689.305415    | -6689.271816     |
| 1D      | 2           | 16        | -6688.682853       | -6689.249613      | -6689.323041    | -6689.290452     |
| 1E      | 16          | 16        | -6689.363419       | -6689.391487      | -6689.391487    | -6689.363419     |
| 2A      | 19          | 19        | -8389.083540       | -8389.122287      | -8389.122287    | -8389.083540     |
| 2B      | 1           | 19        | -8388.268202       | -8388.600756      | -8389.056749    | -8389.026178     |
| 2C      | 1           | 19        | -8388.266365       | -8388.591367      | -8389.062993    | -8389.024431     |

TABLE S2: Hartree-Fock energies in Ha for the  $[\text{Fe}_x\text{S}_4(\text{SCH}_3)_x]^{-2}$  clusters and different geometries studied, computed using a mixed aug-cc-pvDz (Fe, S) cc-pvDz (C, H) basis set. We report results using both ROHF and UHF, with different spin states.

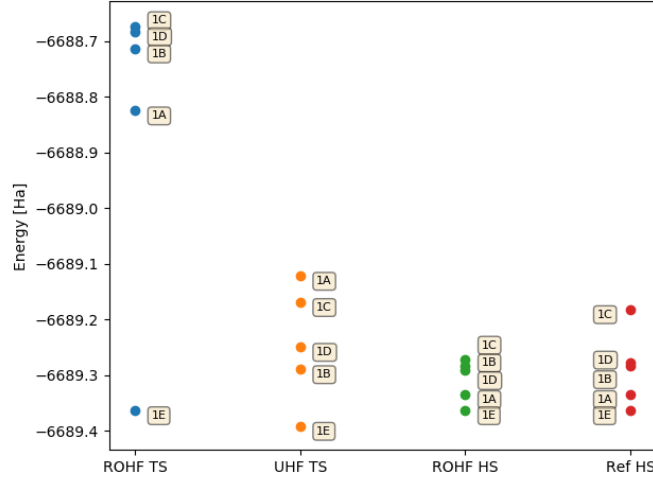

FIG. S1: Hartree-Fock energies in Ha for the five  $[\text{Fe}_3\text{S}_4(\text{SCH}_3)_3]^{-2}$  geometries, computed using a mixed aug-cc-pvDz (Fe,S) cc-pvDz (C,H) basis set. This is the same information as in Tab. S2. Here, TS refers to Target Spin, and HS refers to High Spin.

| cluster | $2S + 1$ | ROHF - canonical | ROHF - localized |
|---------|----------|------------------|------------------|
| 2A      | 19       | -8389.083540     | -8388.655487     |
| 2B      | 19       | -8389.026178     | -8388.488728     |
| 2C      | 19       | -8389.024431     | -8388.488403     |
| 2R      | 19       | -8388.979087     | -8387.533777     |

TABLE S3: ROHF energies in Ha for the high-spin state of the  $[\text{Fe}_x\text{S}_4(\text{SCH}_3)_4]^{-2}$  clusters and different geometries studied, computed using a mixed aug-cc-pvDz (Fe, S) cc-pvDz (C, H) basis set. We report results before and after Pipek-Mezey localization.

and so successively until reaching  $2S + 1 = 2$ . The results are summarized in Fig. S2, together with the low spin ROHF energies for the 1A-D clusters at their corresponding spin multiplicities for reference. This strategy does not improve the low spin ROHF energy appreciably, and thus we decided to keep the HS spin ROHF orbitals as starting points for the CASSCF calculations.

As discussed in the main body of the paper, the Pipek-Mezey localization [23] localization of the ROHF orbitals induces a dramatic energy increase in the high-spin ROHF determinant, due to rotations between open- and closed-shell orbitals. In the paper, we note that the energy penalty associated with localization was  $\sim 0.5$  Ha, Tab. S3 summarizes ROHF energies for the  $\text{Fe}_4$  before and after localization. This is just a different orbital reference to perform the fully correlated CASSCF calculations, advantageous to choose chemically motivated active spaces and to interpret the correlation functions evaluated in the main body of the paper. Further, this localization is a standard

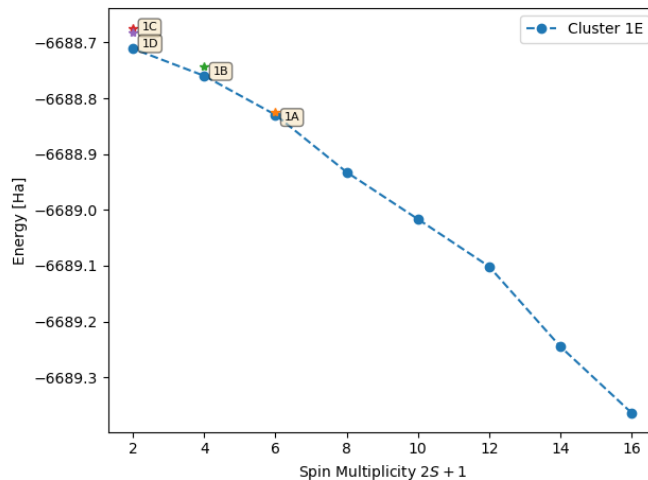

FIG. S2: ROHF energies in Ha for the 1E  $[\text{Fe}_3\text{S}_4(\text{SCH}_3)_3]^{-2}$  cluster, computed using a mixed aug-cc-pvDz (Fe, S) cc-pvDz (C, H) basis set, as a function of the spin multiplicity. We further present the HF energies for the other  $[\text{Fe}_3\text{S}_4(\text{SCH}_3)_3]^{-2}$  clusters for comparison.

procedure used to enhance the convergence of post-HF calculations in complicated systems [24], and that has been applied in particular to the  $\text{Fe}_4$  clusters previously [1]. Indeed, we checked the different CASSCF convergence from these two references (localized vs. canonical ROHF orbitals) for the 2A geometry in the (22e, 20o) and (86e, 52o) active spaces. The results of this test are summarized in Tab. S4, which show that the localized orbitals offer in general a better starting point in terms of the final variational energies. This can be explained by looking at the CASSCF orbitals: those starting from the canonical ROHF basis barely change during the optimization. The canonical orbitals may be a local minimum in the optimization landscape, of which it is apparently hard to escape for these complex systems. These canonical ROHF orbitals are thus not the optimal single-particle basis to describe these clusters. For instance, the Fe-d canonical ROHF orbitals show pairing similar to that of the CASSCF orbitals discussed in the main paper, but instead of grouping the Fe-atoms into the pairs with shortest bond length, the canonical ROHF basis shows pairing between other Fe-pairs. Further, the jump of  $\sim 50$  mHa between the (22e, 20o) and (86e, 52o) active space calculations starting from canonical orbitals (see Tab. S4) only comes upon after the CASSCF optimization includes Fe-p orbitals in the active space, further justifying the active space choices made in the main paper. In essence, this shows how using a localized orbital basis helps with proposing more effective, chemically/physically motivated active spaces.

| Active Space | $2S + 1$ | Can. ROHF start | Loc. ROHF start |
|--------------|----------|-----------------|-----------------|
| (22e, 20o)   | 5        | -8389.087565    | -8389.088122    |
|              | 3        | -8389.087682    | -8389.088318    |
|              | 1        | -8389.087271    | -8389.088439    |
| (86e, 52o)   | 5        | -8389.136037    | -8389.171896    |
|              | 3        | -8389.137031    | -8389.171579    |
|              | 1        | -8389.134055    | -8389.171696    |

TABLE S4: ASCI-SCF energies in Ha for the low spin states of the  $[\text{Fe}_x\text{S}_4(\text{SCH}_3)_4]^{-2}$  cluster in 2A geometry in two active spaces, computed using a mixed aug-cc-pvDz (Fe, S) cc-pvDz (C, H) basis set. We report results starting from the canonical, and Pipek-Mezey localized ROHF basis.

#### IV. CASSCF SPIN CHAINS

In Tab. S5, we report the CASSCF energies for the full spin chains of the  $[\text{Fe}_3\text{S}_4(\text{SCH}_3)_3]^{-2}$  cluster geometries, using a full CI (FCI) solver in a minimal (15e, 15o) active space. This corresponds to the Fe-d orbitals exclusively. We also include results of CASSCF optimizations using DMRG as impurity solver, starting from the CASSCF orbitals.

For comparison, we also provide FCI energies in the ROHF basis for the low spin states (note that the ROHF and CASSCF energies are the same for the high spin state  $2S + 1 = 16$  because of the size of the active space).

| Cluster | $2S + 1$ | FCI-ROHF     | FCI-SCF      | DMRG-SCF<br>( $M = 2000$ ) | DMRG<br>(TRE = $10^{-6}$ ) |
|---------|----------|--------------|--------------|----------------------------|----------------------------|
| 1A      | 16       | -6689.334426 | -6689.334426 |                            |                            |
|         | 14       |              | -6689.335933 |                            |                            |
|         | 12       |              | -6689.337366 |                            |                            |
|         | 10       |              | -6689.338839 |                            |                            |
|         | 8        |              | -6689.340121 | -6689.340274               | -6689.340279               |
|         | 6        | -6689.339015 | -6689.341215 | -6689.341350               | -6689.341341               |
|         | 4        | -6689.338858 | -6689.340781 | -6689.335849               | -6689.340572               |
| 1B      | 2        | -6689.339230 | -6689.340610 | -6689.340328               | -6689.340750               |
|         | 16       | -6689.283679 | -6689.283679 |                            |                            |
|         | 14       |              | -6689.285677 |                            |                            |
|         | 12       |              | -6689.287607 |                            |                            |
|         | 10       |              | -6689.289522 |                            |                            |
|         | 8        |              | -6689.291142 | -6689.291393               | -6689.291372               |
|         | 6        | -6689.289942 | -6689.291607 | -6689.292822               | -6689.292840               |
| 1C      | 4        | -6689.290515 | -6689.292339 | -6689.292800               | -6689.292945               |
|         | 2        | -6689.290791 | -6689.292861 | -6689.289864               | -6689.292976               |
|         | 16       | -6689.271816 | -6689.271816 |                            |                            |
|         | 14       |              | -6689.274084 |                            |                            |
|         | 12       |              | -6689.276320 |                            |                            |
|         | 10       |              | -6689.278336 |                            |                            |
|         | 8        |              | -6689.279943 | -6689.279175               | -6689.280246               |
| 1D      | 6        | -6689.277799 | -6689.281554 | -6689.281728               | -6689.281723               |
|         | 4        | -6689.278867 | -6689.281217 | -6689.279174               | -6689.281680               |
|         | 2        | -6689.279241 | -6689.281637 | -6689.281525               | -6689.281813               |
|         | 16       | -6689.290452 | -6689.290452 |                            |                            |
|         | 14       |              | -6689.292240 |                            |                            |
|         | 12       |              | -6689.294015 |                            |                            |
|         | 10       |              | -6689.295670 |                            |                            |
| 1E      | 8        |              | -6689.297207 | -6689.297370               | -6689.297370               |
|         | 6        | -6689.295966 | -6689.297424 | -6689.297873               | -6689.297879               |
|         | 4        | -6689.296600 | -6689.298314 | -6689.298732               | -6689.298731               |
|         | 2        | -6689.296897 | -6689.298775 | -6689.298614               | -6689.299000               |
|         | 16       | -6689.363419 | -6689.363419 |                            |                            |
|         | 14       |              | -6689.364141 |                            |                            |
|         | 12       |              | -6689.364773 |                            |                            |
| 1F      | 10       |              | -6689.365307 |                            |                            |
|         | 8        |              | -6689.366062 | -6689.366228               | -6689.366213               |
|         | 6        | -6689.365700 | -6689.366541 | -6689.366900               | -6689.366898               |
|         | 4        | -6689.365842 | -6689.366616 | -6689.363073               | -6689.366855               |
|         | 2        | -6689.365980 | -6689.366850 | -6689.365613               | -6689.366911               |

TABLE S5: Full CI (FCI) energies in the ROHF basis, as well as CASSCF energies with FCI solver, for spin states  $2S + 1 = 16 - 2$  starting from the high spin ( $2S + 1 = 16$ ) ROHF orbitals for the  $[\text{Fe}_3\text{S}_4(\text{SCH}_3)_3]^{-2}$  cluster geometries. The active space is (15e, 15o), and the basis set is a mixed aug-cc-pvDz (Fe,S) cc-pvDz (C,H). We mark in blue the spin state for which the geometry was optimized (using BS-DFT), while in green we mark the ground state at the CASSCF level. The second to rightmost column reports CASSCF energies using DMRG as a solver and starting from the full CI CASSCF orbitals, and the last column reports the best DMRG variational energy from those DMRG-SCF orbitals.

The CASSCF energies for the  $\text{Fe}_3$  clusters in Tab. S5 show extremely small gaps, of 1 mHa or below, between successive spin states for the same geometry, a known manifestation of the electrochemical tunability of these transition metal centers [1, 21], which makes them exceptionally hard to treat theoretically. The excellent agreement between full CI and DMRG suggests that even these minute differences can be captured accurately with DMRG. Further, we note that in these  $\text{Fe}_3$  clusters, the orbital optimization is not stabilizing the energy significantly. Indeed, across the different spin states, comparing the first and second columns in Tab. S5, we see that the CASSCF optimization only lowers the energy by a couple of mHa. The Fe-d orbitals alone thus do not contribute significantly to the correlation

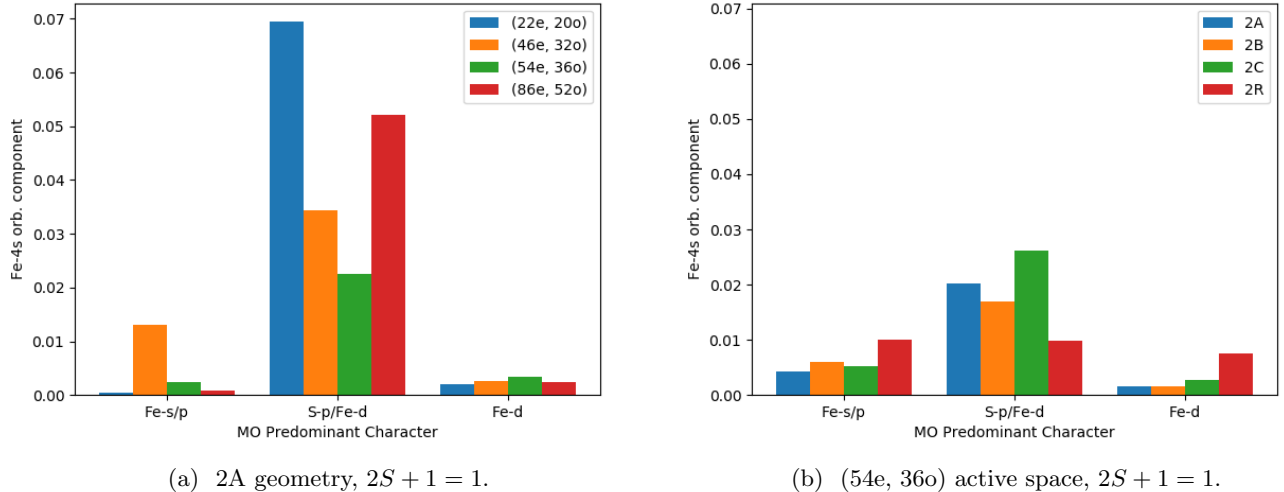

FIG. S3: Relative Fe-4s orbital contribution to the main group of CASSCF optimized orbitals identified in the main paper for the Fe<sub>4</sub> clusters. (a) Different active spaces in the 2A singlet state, (b) (54e, 36o) active space and singlet state for different cluster geometries.

energy, which justifies the small gaps between different spin states, which essentially differ only through the Fe-d electronic configurations.

It is interesting to note that the most stable configuration corresponds to the lowest spin state for almost all Fe<sub>3</sub> geometries, with the exception of 1A, even when 1A-D were obtained by geometry optimization of higher spin states. Only for 1A do the targeted spin state and the actual ground state coincide. Ideally, one would draw from these results a map relating spin ordering to cluster geometry. While our results suggest that such a dependency exists, seeing how 1A has a more stable sextet than singlet both within full CI and subsequent DMRG CASSCF, the small gaps preclude any definitive statement in this direction.

| Cluster | $2S + 1$ | DMRG-SCF(M = 2000) | DMRG(TRE = $10^{-6}$ ) |
|---------|----------|--------------------|------------------------|
| 2A      | 5        | -8389.088135       | -8389.088093           |
|         | 3        | -8389.088485       | -8389.088490           |
|         | 1        | -8389.087962       | -8389.087967           |
| 2B      | 5        | -8389.038593       | -8389.038703           |
|         | 3        | -8389.039388       | -8389.039372           |
|         | 1        | -8389.039751       | -8389.039841           |
| 2C      | 5        | -8389.032837       | -8389.034725           |
|         | 3        | -8389.033106       | -8389.034522           |
|         | 1        | -8389.037192       | -8389.037287           |

TABLE S6: DMRG results for the Fe<sub>4</sub> clusters and CAS(22,20).

## V. FE-4S ORBITAL COMPONENT IN CASSCF MOLECULAR ORBITALS

In the main paper, we ascribe the dynamical role of the bridging S-p orbitals on the one hand to the double-exchange mechanism, and on the other to their interactions with the essentially empty Fe-4s orbitals. We corroborate the presence double-exchange mechanism in the main paper, by studying charge and spin fluctuations between the Fe-d and S-p orbitals through charge density and spin-spin correlation plots, as well as by looking at the mutual information between the orbitals on this atoms. To support the latter part of the interpretation, in Fig. S3 we report the relative contribution of the Fe-4s atomic orbitals (from the aug-cc-pVDZ Fe basis set) into the three main groups of CASSCF optimized molecular orbitals: the Fe-p/s orbitals, the S-p/Fe-d hybrid orbitals, and the Fe-d orbitals.

We show these contributions for the different active spaces considered in the main paper and the 2A geometry with

| Calculation     | $2S + 1$ | ASCI      | ASCI+PT2 extrapol.       | DMRG<br>(TRE = $5 \cdot 10^{-6}$ ) |
|-----------------|----------|-----------|--------------------------|------------------------------------|
| CAS - ROHF      | 5        | -6.809861 | $-6.954208 \pm 0.024262$ | -6.984349                          |
|                 | 3        | -6.795443 | $-6.942742 \pm 0.016892$ | -6.985358                          |
|                 | 1        | -6.790068 | $-6.933416 \pm 0.011166$ | -6.986202                          |
| CAS - roDFT [1] | 5        | -6.356089 | $-6.520918 \pm 0.044194$ | -6.700676 <sup>a</sup>             |
|                 | 3        | -6.338865 | $-6.479879 \pm 0.034909$ | -6.706775 <sup>a</sup>             |
|                 | 1        | -6.300973 | $-6.547974 \pm 0.025194$ | -6.711691 <sup>a</sup>             |
| CASSCF @ ROHF   | 5        | -7.095949 | $-7.108954 \pm 0.003143$ | -7.104995                          |
|                 | 3        | -7.096320 | $-7.109667 \pm 0.002459$ | -7.106331                          |
|                 | 1        | -7.096661 | $-7.109896 \pm 0.002386$ | -7.105501                          |

<sup>a</sup> TRE =  $5 \cdot 10^{-5}$

TABLE S7: CAS and CASSCF energies ( $E - 8380.0$  Ha) using ASCI and DMRG for a (54e, 36o) active space in the 2R  $[\text{Fe}_4\text{S}_4(\text{SCH}_3)_4]^{-2}$  geometry, in the def2-svp basis set. The CAS calculations are performed in the using the high spin ( $2S + 1 = 19$ ) ROHF and roDFT (BP86 functional) orbitals, localized with Pipek-Mezey. The CASSCF calculations start from the localized ROHF orbitals. The ASCI-PT2 extrapolations to the FCI limit use a linear extrapolation from calculations with  $5 \cdot 10^5$ ,  $1 \cdot 10^6$ ,  $2 \cdot 10^6$ ,  $5 \cdot 10^6$  determinants. The error bars correspond to the standard deviation of the linear fit, and are thus just a measure of the extrapolation error alone.

singlet state in Fig S3a, and for the (54e, 36o) active space, singlet state for the different geometries of  $\text{Fe}_4$  clusters in Fig. S3b. We see that the Fe-4s atomic orbitals play only a small role in all CASSCF optimized molecular orbitals (MOs), but their contribution to the S-p-based MOs is larger than in the rest of the active space. While there is some dependency of the actual magnitude on the active space size and geometry, the conclusion that the S-p orbitals couple to the Fe-4s orbitals is valid.

## VI. 2R $\text{Fe}_4$ GEOMETRY WITH DEF2-SVP BASIS SET

In order to provide a direct comparison to the previous literature, we performed calculations on the 2R  $\text{Fe}_4$  geometru using the def2-svp basis set (384 basis functions). This should make our results directly comparable to those in Ref. [1]. Similarly with the (aug)-cc-pVDZ calculations, we performed an ROHF for the highest spin state  $2S + 1 = 19$ , and applied Pipek-Mezey optimization to obtain the initial orbital basis for the subsequent CASSCF calculation. We report in Tab. S7 the ground state energies for spin states  $2S + 1 = 1, 3, 5$  using the (54e, 36o) active space described in the main paper, for ROHF, roDFT and CASSCF orbitals using the SP-ASCI and DMRG solvers. The roDFT orbitals are obtained using the BP86 functional in a high-spin ( $2S + 1 = 19$ ) calculation of the *all ferric* state, i.e. the charge neutral  $[\text{Fe}_4\text{S}_4(\text{SCH}_3)_4]$  cluster, as was performed in Ref. [1]. We note that our absolute energies do not agree with Ref. [1], although our DMRG energy gaps agree well. While the disagreement of the absolute energies is puzzling, only the gaps are physical quantities, and thus we trust our results are significant and representative of the true behavior of these clusters. The perturbative extrapolation from the ASCI wave functions is larger in these def2-SVP results ( $\sim 10$  mHa) than in the (aug)-ccpVDZ calculations in the main paper ( $\sim 5$  mHa), which suggests a more prominent role of the dynamical correlation in the CASSCF optimized orbital basis obtained in the smaller basis set.

In general, Tab. S7 shows the same trend we have discussed in the main paper: ASCI struggles to converge in the mean-field orbital bases (ROHF and roDFT), with large perturbative corrections, extrapolation errors and energy gaps between consecutive spin states, as well as a poor agreement with the DMRG result (which do present  $\sim 1$  mHa gaps in agreement with the literature). Notwithstanding these difficulties, it can be used as approximate CAS solver within the CASSCF orbital optimization to obtain much more reliable energies, in good agreement with the DMRG values and showing reasonable energy gaps.

Comparing the CAS energies with mean-field orbitals in Tab. S7, we observe that the ROHF orbitals from the reduced (anyonic) cluster are a variationally better starting point than the roDFT ones for the all ferric oxidation state. Indeed, both the ASCI and DMRG energies starting from ROHF orbitals are significantly lower than the ones starting from roDFT. Furthermore, even the energy gaps between neighbouring spin states seem to be more accurate in the ROHF basis, at least within the DMRG treatment, the gaps computed from the roDFT basis being too large. Similarly, using the ROHF orbitals as starting point, the more complex mixed (aug)-cc-pVDZ basis set provides energies almost 2 Ha lower than the def2-SVP basis set, as shown in the main paper. This is not a surprise, given the introduction of higher angular momentum orbitals.

It is interesting to note that, in contrast with all CASSCF optimizations performed in the (aug)-cc-pVDZ basis set, the DMRG-SCF optimization performed after with the ASCI-SCF orbitals did result in a noticeable energy lowering of  $\sim 10$  mHa (comparing extrapolated ASCI+PT2 energies to the DMRG ones). This is not necessarily a statement about the different solvers, since the CASSCF optimization landscape with this many basis functions (384), and this large an active space (54e, 36o), is prone to local minima. As noted in the main paper, we cannot guarantee at any point to have reached the true global minimum in the orbital optimization, we can only be certain to be at a stable local minimum. Indeed, we were able to further optimize the ASCI-SCF energies by “shaking” the single-particle orbitals away from their stable local minimum, resulting in the values in Tab. S7, which are in excellent agreement with the DMRG results. This “shaking” was done by performing an inexpensive ASCI-SCF calculation starting from the previously optimized orbitals, *without* enforcing total-spin conservation symmetry within the SP-ASCI framework. This results in single-particle orbitals different enough from the previously optimized ones, such that subsequent SP-ASCI-SCF optimizations can escape the local minimum, and improve in energy. Despite the agreement between ASCI and DMRG observed throughout this study, the fact remains that DMRG and ASCI use different wave function Ansätze, and hence may describe efficiently non-intersecting regions of the many-body Hilbert space. As a result, there is no clear way to decide, *a priori*, which one of the two solvers, if any, is likely to produce a variationally better set of single-particle orbitals. This just further emphasizes the importance of performing studies comparing different methods when dealing with strongly correlated systems.

To complete the 2R def2-SVP results, we report the largest spin-gap, between the singlet and  $2S + 1 = 19$  states, in Tab. S8.

| Geometry | $2S + 1 = 1$ | $2S + 1 = 19$ | Spin Gap [mHa]    |
|----------|--------------|---------------|-------------------|
| 2R       | -7.081655    | -7.068382     | -13.273 (-23.823) |

TABLE S8: ASCI energies ( $E - 8380.0$  Ha) using SP-ASCI as solver for the 2R Fe<sub>4</sub> cluster geometry in the  $2S + 1 = 1$  and  $2S + 1 = 19$  spin states in the (54e, 36o) active space and def2-SVP basis. The energies are computed using the CASSCF orbitals optimized for the singlet state. The last column reports the spin gap in mHa, computed as  $E_0^{2S+1=1} - E_0^{2S+1=19}$ . The numbers in parenthesis are the spin gaps computed in the localized ROHF basis using DMRG.

## VII. CASSCF WITH DIFFERENT BASIS SETS

Given the complexity of the CASSCF optimization problem, it becomes important to check the effect of the basis set choice on the final energy gaps and extrapolation errors. While the main paper already contains some data on this, presenting results for the 2R geometry in the def2-SVP and (aug)-cc-pVDZ basis sets, we want to complement this comparison by presenting a case example with two basis sets of similar number of basis functions. We do so briefly here, on the example of the 2A geometry in the (aug)-cc-pVDZ basis set used in the main paper, and the def2-TZVP basis set. Rather than concentrating on the number of basis functions, which necessarily affects the optimization since it determines the dimensionality of the objective function, we want to consider the nature of those basis functions. In particular, the mixed aug-cc-pVDZ (Fe,S) cc-pVDZ (C,H) basis set contains high angular momentum functions, which introduce near linear dependencies, likely to result in a higher proclivity for falling into local minima. It seems plausible to expect that the def-TZVP basis set, which has a comparable number of basis functions (672 vs. 568) but comparatively less high angular momentum functions, should provide for a simpler optimization. We report CASSCF energies for the 2A geometry and (54e, 36o) active space for both basis sets in Tab. S9, using SP-ASCI as solver, as well as extrapolated SP-ASCI+PT2 energies.

From Tab. S9, we see fairly consistent results with both basis sets: sub mHa energy gaps between the different spin states, both at the CASSCF and extrapolated ASCI+PT2 level of theory. The mixed aug-cc-pVDZ (Fe,S) cc-pVDZ (C,H) results are  $\sim 11$  mHa lower in energy than the def-TZVP ones, which is likely at least partially due to the diffuse orbitals improving the description of the anionic oxidation state. Regarding the optimization complexity, however, both CASSCF sets are similarly hard to perform, and need exchanging orbitals between the spin states to escape local minima.

---

[1] S. Sharma, K. Sivalingam, F. Neese, and G. K.-L. Chan, “Low-energy spectrum of iron-sulfur clusters directly from many-particle quantum mechanics,” *Nature chemistry* **6**, 927–933 (2014).

| Basis Set         | $2S + 1$ | CASSCF<br>SP-ASCI-SCF | ASCI+PT2 extrapol.<br>SP-ASCI |
|-------------------|----------|-----------------------|-------------------------------|
| (aug)-<br>cc-pVDZ | 5        | -8389.150451          | -8389.155331 $\pm$ 0.000981   |
|                   | 3        | -8689.150856          | -8389.155357 $\pm$ 0.000843   |
|                   | 1        | -8389.150950          | -8389.155423 $\pm$ 0.000681   |
| def-TZVP          | 5        | -8389.141441          | -8389.144527 $\pm$ 0.000618   |
|                   | 3        | -8389.141496          | -8389.144588 $\pm$ 0.000612   |
|                   | 1        | -8389.141758          | -8389.144753 $\pm$ 0.000573   |

TABLE S9: CASSCF and extrapolated results using SP-ASCI (54e, 36o) active space in the 2A Fe<sub>4</sub> cluster geometry, starting from the high spin ( $2S + 1 = 19$ ) ROHF orbitals, localized with Pipek-Mezey, using two different basis sets: the mixed aug-cc-pVDZ (Fe,S) cc-pVDZ (C,H) basis set used in the rest of this work, and the def-TZVP basis set. The CASSCF energies correspond to SP-ASCI calculations with  $5 \cdot 10^6$  determinants. These correspond to the final step of a series of SP-ASCI-SCF calculations starting at  $1 \cdot 10^5$  determinants, and progressively increasing the number of determinants to improve the orbitals sequentially. The ASC+PT2 extrapolated results are estimating the FCI limit, using a linear extrapolation from calculations with  $5 \cdot 10^5$ ,  $1 \cdot 10^6$ ,  $2 \cdot 10^6$ ,  $5 \cdot 10^6$  determinants, starting from the orbitals obtained from the SP-ASCI-SCF with  $5 \cdot 10^6$  determinants. The error bars correspond to the standard deviation of the linear fit, and are thus just a measure of the extrapolation error alone.

- [2] B. Huron, J. Malrieu, and P. Rancurel, “Iterative perturbation calculations of ground and excited state energies from multiconfigurational zeroth-order wavefunctions,” *The Journal of Chemical Physics* **58**, 5745–5759 (1973).
- [3] S. Evangelisti, J.-P. Daudey, and J.-P. Malrieu, “Convergence of an improved cipsi algorithm,” *Chemical Physics* **75**, 91–102 (1983).
- [4] F. Illas, J. Rubio, J. Ricart, and P. Bagus, “Selected versus complete configuration interaction expansions,” *The Journal of chemical physics* **95**, 1877–1883 (1991).
- [5] P.-O. Löwdin, “Quantum theory of many-particle systems. i. physical interpretations by means of density matrices, natural spin-orbitals, and convergence problems in the method of configurational interaction,” *Physical Review* **97**, 1474 (1955).
- [6] P.-O. Löwdin, “Quantum theory of cohesive properties of solids,” *Advances in Physics* **5**, 1–171 (1956).
- [7] P.-O. Löwdin and H. Shull, “Natural orbitals in the quantum theory of two-electron systems,” *Physical Review* **101**, 1730 (1956).
- [8] E. R. Davidson, “Properties and uses of natural orbitals,” *Reviews of Modern Physics* **44**, 451 (1972).
- [9] D. S. Levine, D. Hait, N. M. Tubman, S. Lehtola, K. B. Whaley, and M. Head-Gordon, “Casscf with extremely large active spaces using the adaptive sampling configuration interaction method,” *Journal of chemical theory and computation* **16**, 2340–2354 (2020).
- [10] Q. Zhao, X. Zhang, J. M. P. Martirez, and E. A. Carter, “Benchmarking an embedded adaptive sampling configuration interaction method for surface reactions: H<sub>2</sub> desorption from and ch<sub>4</sub> dissociation on cu (111),” *Journal of Chemical Theory and Computation* (2020).
- [11] N. M. Tubman, J. Lee, T. Y. Takeshita, M. Head-Gordon, and K. B. Whaley, “A deterministic alternative to the full configuration interaction quantum monte carlo method,” *J. Chem. Phys.* **145**, 044112 (2016).
- [12] N. M. Tubman, D. S. Levine, D. Hait, M. Head-Gordon, and K. B. Whaley, “An efficient deterministic perturbation theory for selected configuration interaction methods,” *arXiv preprint arXiv:1808.02049v1* (2018).
- [13] N. M. Tubman, C. Mejuto-Zaera, J. M. Epstein, D. Hait, D. S. Levine, W. Huggins, Z. Jiang, J. R. McClean, R. Babbush, M. Head-Gordon, *et al.*, “Postponing the orthogonality catastrophe: efficient state preparation for electronic structure simulations on quantum devices,” *arXiv preprint arXiv:1809.05523* (2018).
- [14] C. Mejuto-Zaera, N. M. Tubman, and K. B. Whaley, “Dynamical mean field theory simulations with the adaptive sampling configuration interaction method,” *Physical Review B* **100**, 125165 (2019).
- [15] D. Hait, N. M. Tubman, D. S. Levine, K. B. Whaley, and M. Head-Gordon, “What levels of coupled cluster theory are appropriate for transition metal systems? a study using near-exact quantum chemical values for 3d transition metal binary compounds,” *Journal of chemical theory and computation* **15**, 5370–5385 (2019).
- [16] C. Mejuto-Zaera, G. Weng, M. Romanova, S. J. Cotton, K. B. Whaley, N. M. Tubman, and V. Vlček, “Are multi-quasiparticle interactions important in molecular ionization?” *arXiv-preprint 2009.02401* (2020).
- [17] N. M. Tubman, C. D. Freeman, D. S. Levine, D. Hait, M. Head-Gordon, and K. B. Whaley, “Modern approaches to exact diagonalization and selected configuration interaction with the adaptive sampling ci method,” *Journal of chemical theory and computation* **16**, 2139–2159 (2020).
- [18] J. J. Eriksen, T. A. Anderson, J. E. Deustua, K. Ghanem, D. Hait, M. R. Hoffmann, S. Lee, D. S. Levine, I. Magoulas, J. Shen, *et al.*, “The ground state electronic energy of benzene,” *The journal of physical chemistry letters* **11**, 8922–8929 (2020).
- [19] B. S. Fales, E. G. Hohenstein, and B. G. Levine, “Robust and efficient spin purification for determinantal configuration interaction,” *Journal of Chemical Theory and Computation* **13**, 4162–4172 (2017).
- [20] T. Applencourt, K. Gasperich, and A. Scemama, “Spin adaptation with determinant-based selected configuration interaction,” *arXiv preprint arXiv:1812.06902* (2018).

- [21] G. Li Manni, W. Dobrautz, N. A. Bogdanov, K. Guther, and A. Alavi, “Resolution of low-energy states in spin-exchange transition-metal clusters: Case study of singlet states in [fe (iii) 4s4] cubanes,” (2020).
- [22] T. Helgaker, P. Jorgensen, and J. Olsen, *Molecular Electronic Structure Theory* (Wiley, New York, 2000).
- [23] J. Pipek and P. G. Mezey, “A fast intrinsic localization procedure applicable for abinitio and semiempirical linear combination of atomic orbital wave functions,” *The Journal of Chemical Physics* **90**, 4916–4926 (1989).
- [24] L. Bytautas, J. Ivanic, and K. Ruedenberg, “Split-localized orbitals can yield stronger configuration interaction convergence than natural orbitals,” *The Journal of chemical physics* **119**, 8217–8224 (2003).
